# Supplementary material for: Cross-city Few-Shot Traffic Forecasting via Traffic Pattern Bank
Source: arXiv:2308.09727 source file (2023-08-17)
Supplement: Supplementary file 1 [file supplement.tex]

\appendix
% \section{Supplementary Material}

\section{Pre-training Stage}

% \subsection{Implementation}
\noindent{\textbf{Implementation}}
The hyper-parameters of the Pre-training stage are listed in Table~\ref{tab:sup_predetail}. 
The positional embedding is initialized with the uniform distribution $\mathcal{U}(-0.02,0.02)$.
During training, we divide the input three-city source data into 70\%, 20\%, and 10\% parts randomly and use them in training, validation, and testing respectively.
% The model with the minimum validation error will be used in the downstream stage to generate traffic patch embeddings.

\begin{table}[hp]
    \caption{Hyper-parameters of Pre-training}
    \label{tab:sup_predetail}
    \centering
    % \resizebox{}{}{}
    \begin{tabular}{c|c}
    \toprule
       Parameter  & Value \\
    \midrule
       Batch size  & 4 \\
       Optimizer & Adam \\
       Learning rate & 0.0001\\
       $\beta_1$, $\beta_2$ & 0.9,0.999\\
       % $\epsilon$ & 1e-08\\
    \midrule
       \# of patches of input & 24 \\
       \# of time steps per patch & 12\\
        Mask ratio & 75\% \\
    \midrule
        Patch embedding size & 128\\
       % Positional embedding size & 128\\
       Positional embedding dropout & 0.1\\
       \# of transformer layers of encoder & 4\\
       \# of transformer layers of decoder & 1\\
    \bottomrule
    \end{tabular}
\end{table}

% \subsection{Results}
\noindent{\textbf{Training}}
The learning curve of the four pre-training processes is shown in Fig.~\ref{fig:supprecurve}. 
The Mean Square Error on validation data is reported, which shows the training process is converged.
Moreover, the reconstitution error of test data is shown in Table~\ref{tab:sup_test}.
This error can be used to determine whether the pretrain stage is properly conducted.

% The error is relatively low, which shows that the pre-trained encoder learns from the traffic data well.   
% The error is larger than the forecasting error in Table~\ref{tab:performance}, which indicates the pre-train task is challenging due to the high mask ratio.

\begin{figure}[hp]
    \centering
    \includegraphics[width=0.93\linewidth]{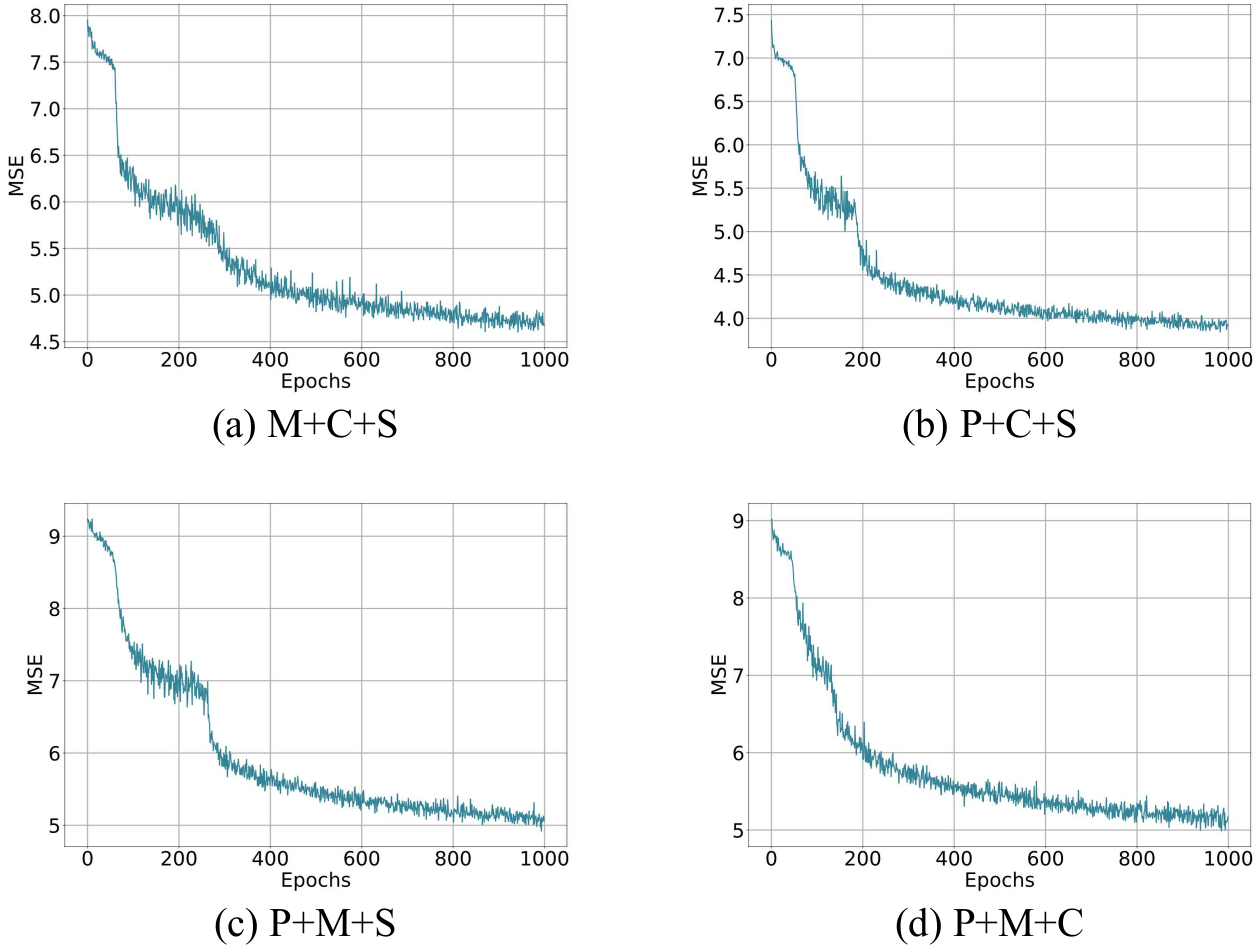}
    \caption{The Mean Square Error on the validation set during the Pre-training stage of each source data. Datasets of source data are denoted by their first letter, e.g., M+C+S represents pre-training in the joint source data of \textit{METR-LA}, \textit{Chengdu}, and \textit{Shenzhen}}
    \label{fig:supprecurve}
    % \vspace{-0.2cm}
\end{figure}

\begin{table}[htb]
\caption{The error of the Pre-training.
The average reconstruction error of the masked patches on test data is reported.
"$\backslash$" represents this dataset is not included in the source data.}
\label{tab:sup_test}
\resizebox{0.9\linewidth}{!}{
% \begin{tabular}{c|c c|c c|c c||c c|c c|c c}
\begin{tabular}{c|c c c|c c c}
\toprule
 % a&a&a&a&a&a&a&a&a&a&a&a\\

& \multicolumn{3}{c|}{\textbf{PEMS-BAY}} & \multicolumn{3}{c}{\textbf{METR-LA}} \\

\cline{2-7}
& RMSE & MAE & MAPE & RMSE & MAE & MAPE \\
\midrule
\midrule

M+C+S  & $\backslash$ & $\backslash$ & $\backslash$ & 7.031 & 4.042 & 10.855  \\
P+C+S &  4.416 & 2.374 & 5.131  & $\backslash$ & $\backslash$ & $\backslash$ \\
P+M+S &  4.611 & 2.424 & 5.563  & 7.071 & 4.015 & 10.944  \\
P+M+C &  4.496 & 2.397 & 5.335  & 7.122 & 4.034 & 10.935  \\
\midrule
\midrule
& \multicolumn{3}{c|}{\textbf{Chengdu}} & \multicolumn{3}{c}{\textbf{Shenzhen}}\\
\cline{2-7}
& RMSE & MAE & MAPE & RMSE & MAE & MAPE \\
\midrule
\midrule
M+C+S  & 3.659 & 2.547 & 10.642 & 3.564 & 2.387 & 9.779 \\
P+C+S  & 3.648 & 2.535 & 10.572 & 3.547 & 2.392 & 9.724 \\
P+M+S & $\backslash$ & $\backslash$ & $\backslash$ & 3.515 & 2.347 & 9.661 \\
P+M+C & 3.699 & 2.581 & 10.794 & $\backslash$ & $\backslash$ & $\backslash$ \\
\bottomrule
\bottomrule

\end{tabular}
}
\end{table}

\noindent{\textbf{Visualization}}
\begin{figure}[htp]
    \centering
    \includegraphics[width=0.98\linewidth]{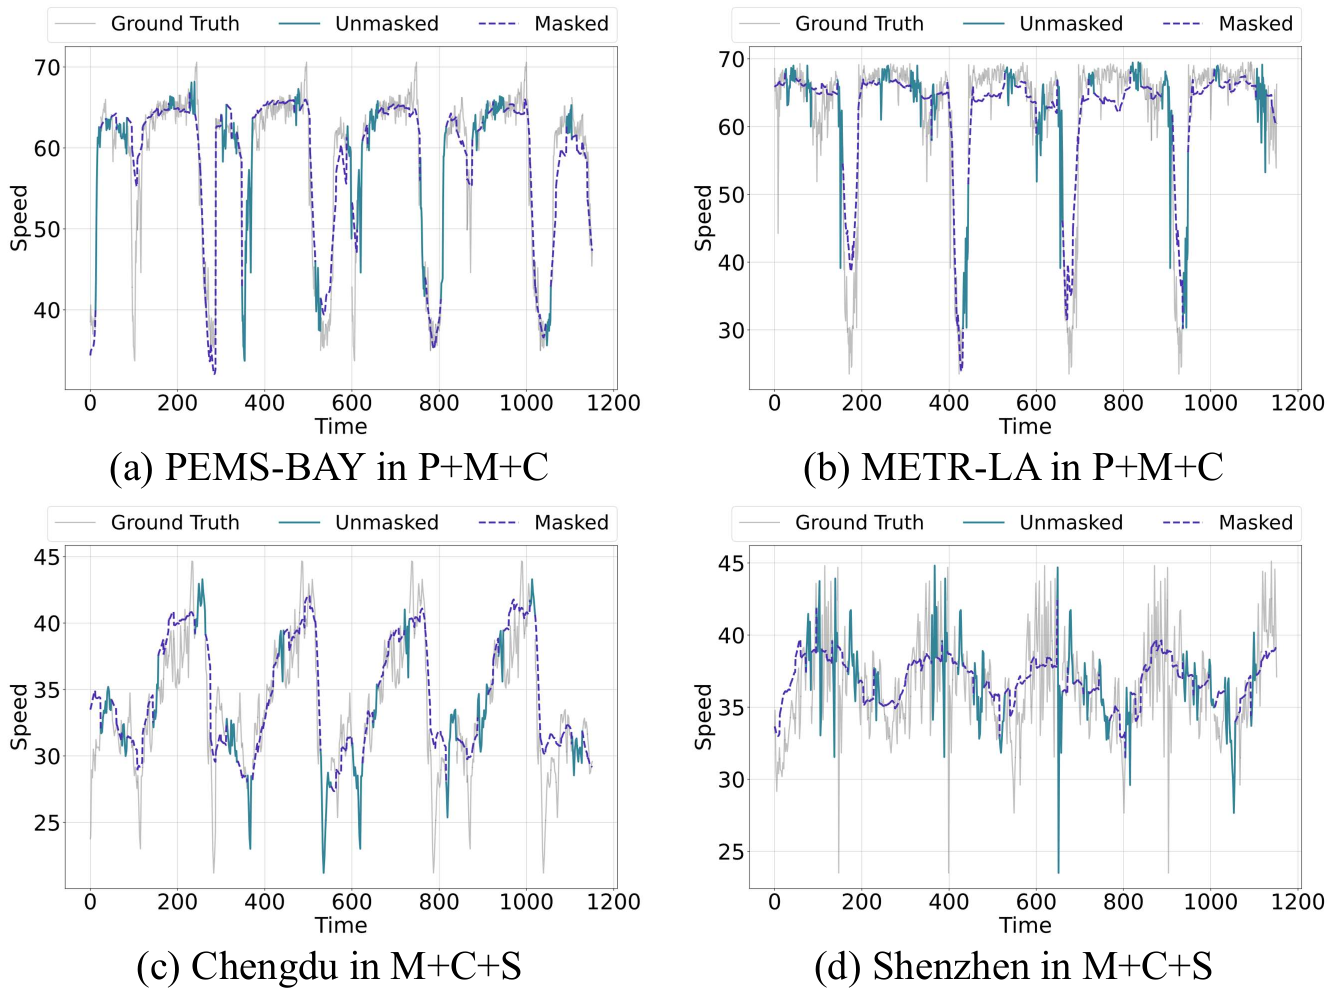}
    % \caption{Fine-grained Deep Traffic Inference (FDTI) architecture for multi-step inference. }
    \caption{The visualization of patch reconstruction in the Pre-training stage. The gray line is the ground truth data, and the blue line and purple dash represent the unmasked data and masked data respectively.}
    \label{fig:supprevis}
    % \vspace{-0.2cm}
\end{figure}

Fig.~\ref{fig:supprevis} visualize the result of reconstructing masked patches.
We randomly select a node and then randomly select a four-day time series on this node to visualize.
We could observe that though most of the patches are masked, the model is still able to learn the general dynamics of the traffic patches.
This benefits the cross-city few-shot forecasting setting because the encoder is robust and general enough to generate traffic patterns used in the target city.

\section{Pattern Generation Stage}

\begin{figure*}[thp]
    \centering
    \includegraphics[width=0.95\linewidth]{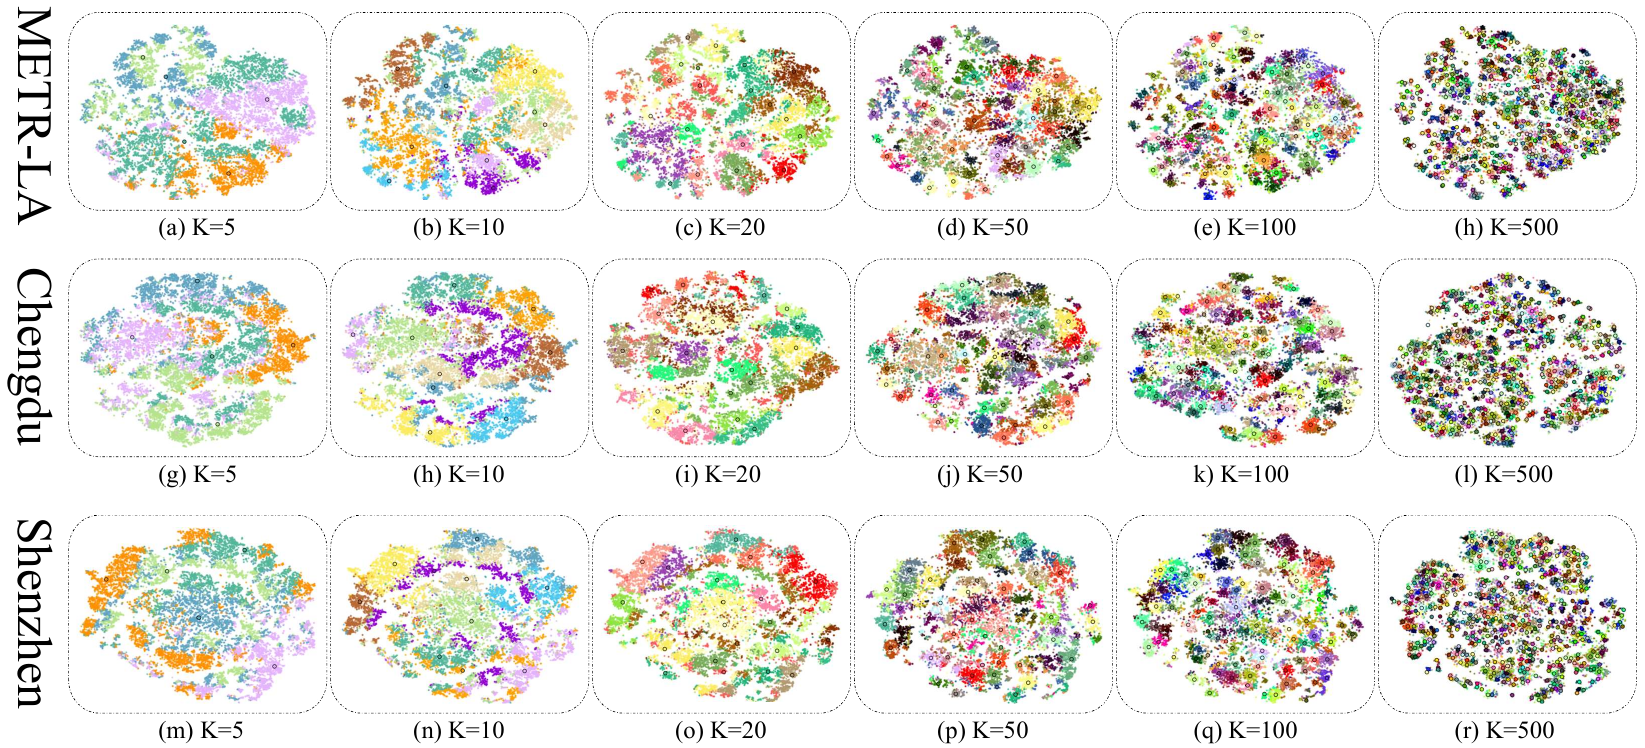}
    % \caption{Fine-grained Deep Traffic Inference (FDTI) architecture for multi-step inference. }
    \caption{The TSNE visualizations of the embeddings of traffic patch and pattern with different K on three traffic datasets. The colored dots indicate the traffic patch embeddings belonging to different clusters. The black circles indicate the traffic pattern embeddings, which are the centroids of different clusters.}
    \label{fig:supclusters}
    % \vspace{-0.2cm}
\end{figure*}

\noindent{\textbf{Implementation}}
% \subsection{Implementation}
We use the traffic patch series of the source data to generate traffic patch embeddings. As is the Pre-training stage, the number of patches of the input of the transformer encoder is 24 and each patch contains 12 time steps. 
Then, to reduce the time complexity, the enormous traffic patch embeddings are sampled with a sample ratio of 0.1.
KMeans clustering algorithm with cosine distance is then applied to the traffic patch embeddings to generate a traffic pattern bank.

% \subsection{Visualization}
\noindent{\textbf{Visualization}}
The clustering results of \textit{METR-LA}, \textit{Chengdu}, and \textit{Shenzhen} are visualized in Fig.~\ref{fig:supclusters}, which shows the clusters with small K are more distinct from other clusters while clusters with larger K are more similar to each other.

\section{Forecasting Stage}

\begin{table}[hp]
    \caption{Hyper-parameters of Pre-training}
    \label{tab:sup_finaldetail}
    \centering
    % \resizebox{}{}{}
    \begin{tabular}{c|c}
    \toprule
       Parameter  & Value \\
    \midrule
        Framework of meta-training & \textit{Reptile}~\cite{nichol2018first} \\
       Batch size of meta-training & 16 \\
        Optimizer of meta-training & SGD \\
       Learning rate of support task $\alpha$  & 0.0005 \\
       Learning rate of query task $\beta$ & 0.0005 \\
       
    \midrule
       Batch size of fine-tuning & 16\\
       Optimizer of fine-tuning & AdamW \\
       Learning rate of fine-tuning & 0.001 \\
       $\beta_1$, $\beta_2$ & 0.9, 0.999\\
       Weight decay & 0.01\\
    \bottomrule
    \end{tabular}
    \vspace{-.3cm}
\end{table}

\noindent{\textbf{Implementation}}
% \subsection{Implementation}
The hyper-parameters of the Forecasting stage are listed in Table~\ref{tab:sup_finaldetail}.
The source data is used in the Forecasting stage, in which use Reptile meta-training framework to get better initial parameters of the learnable modules.
Then these modules are fine-tuned on the few-shot target data. 
Note that in this stage, the traffic pattern bank is fixed and will not be updated by the gradients.

\begin{figure}[htp]
    \centering
    \includegraphics[width=0.98\linewidth]{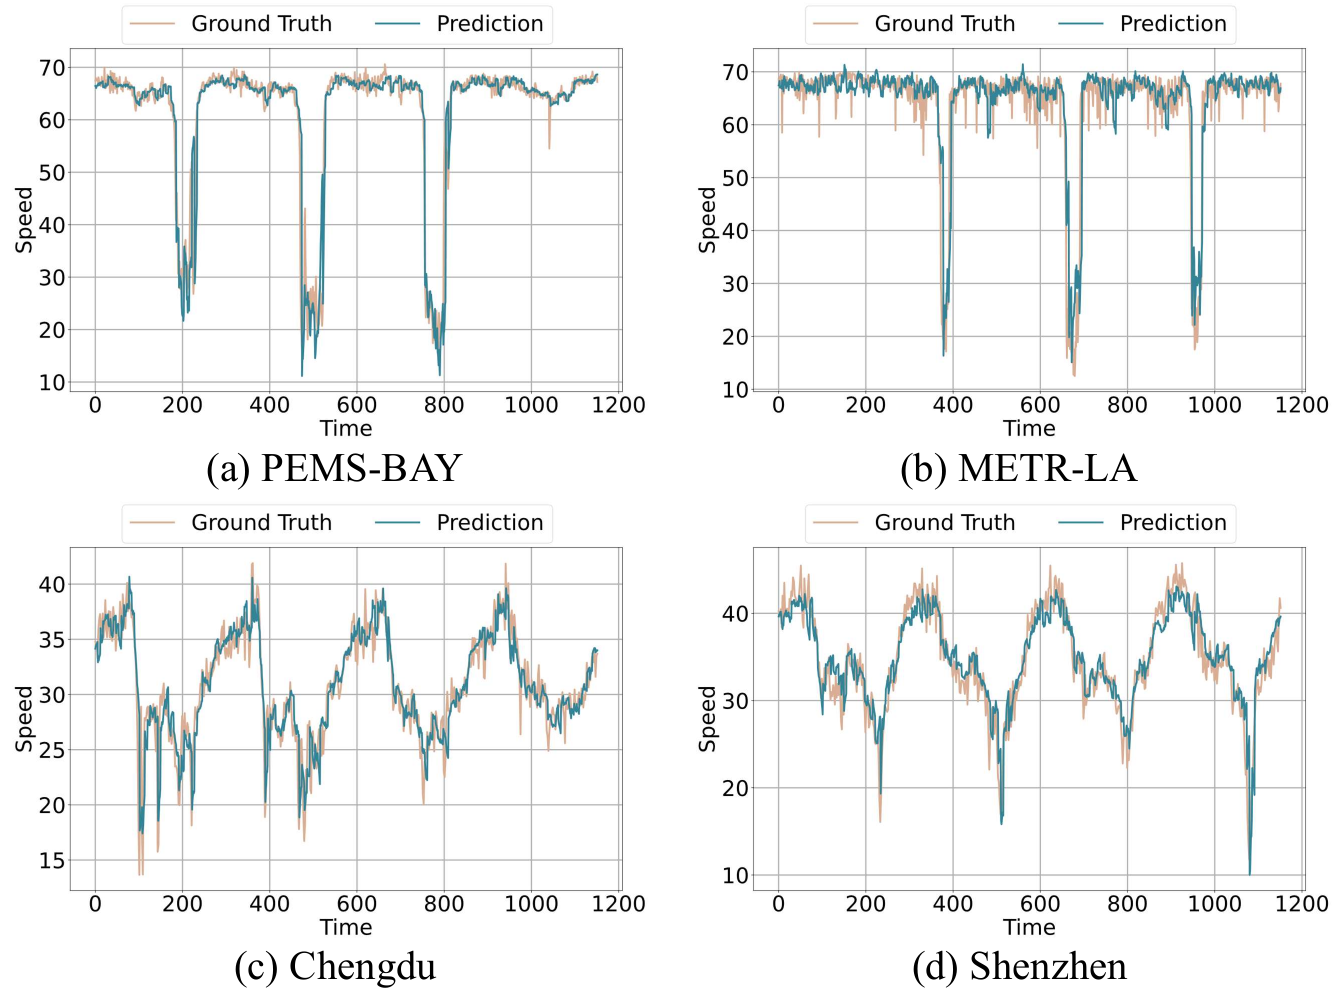}
    % \caption{Fine-grained Deep Traffic Inference (FDTI) architecture for multi-step inference. }
    \caption{The visualization of the Forecasting stage on four datasets.}
    \label{fig:sup_finalvis}
    \vspace{-0.2cm}
\end{figure}

\noindent{\textbf{Visualization}}
% \subsection{Visualization}
The visualization of the results of the Forecasting stage is shown in Fig.~\ref{fig:sup_finalvis}.
We randomly select a node and then randomly select a 4-day time series on this node to visualize.
We could observe that the model makes accurate predictions and furthermore fit the drastic change of the time series, which demonstrates that the model captures the proper traffic patterns and perform well on the cross-city few-shot traffic forecasting task.
% \footnote{The code of TPB is in https://drive.google.com/drive/folders/1UrKTgR27YmP9PjJ-FWv4SCDH3zUxtc5R?usp=sharing. Note that the "-" is included in the url.}

% \section{Baseline Implementation Details}
